# Supplementary material for: SoftNull: Many-Antenna Full-Duplex Wireless via Digital Beamforming
Source: arXiv:1508.03765 source file (2017-03-26)
Supplement: Supplementary file 1 [file measurementAppendix.tex]

%\subsection*{Hardware and Software Apparatus}
\label{sec:implementation}

We implemented a custom baseband design to facilitate realtime measurements. The design enables each radio to transmit a pilot signal in sequence, while all other radios listen.   Along with each pilot, reference symbols to validate the measurements are also sent. This training sequence enables the entire $\numTotal \times \numTotal$ self-interference channel matrix to be in less than 15 $\mu$s per radio, or roughly 1 ms for all 72 antennas. 
Thus  accurate channels are collected within the channel coherence, regardless of environmental changes.
For pilots we use the standard 802.11 preamble, which consists of 20 MHz short training symbols (STSs) and long training symbols (LTSs).
To facilitate channel measurement to both the users and across the base station simultaneously, we implemented a custom automatic gain control (AGC), which does \emph{not} change the radio's Maxim 2829 tranceiver's low noise amplifier (LNA) gain. Altering the LNA gain since it substantially changes the phase of the measured channel. %, and instead only alters the Maxim's ``baseband" gain, which we verified does not affect the channel measurements.
Instead, our custom AGC only alters the Maxim 2829 tranceiver's baseband gain, which  does not affect the measurement phase.%, only the amplitude, which we normalize based on the gain setting.
%However, in order to reduce the delay we implemented a custom automatic gain control, which adjusts the gain for each pilot using only 3 802.11 STSs, rather than the typical 10 (by leveraging the base stations internal time synchronization).
%Additionally our AGC is configured to \emph{not} adjust the Maxim 2829 tranceivers' ``RF" gain, since it substantially alters the phase of the measured channel, and instead only alters the Maxim's ``baseband" gain, which we verified does not affect the channel measurements.
%This allows us to increase the dynamic range of our channel measurements by roughly 60dB, drastically increasing the EVM...
% (called baseband gain, since adjusting the LNA gain affects the phase of the channel measurements, and as such renders the channel measurements unusable for beamforming.
%Our custom AGC is therefore able to drastically increase the noi of our measurements (by over X10X \% for the antennas spaced furthest apart), by helping place signals within the dynamic range of the ADC, without compromising phase accuracy.

%To collect user channels we use a final WARP board which is also time-frequency synchronized with the base station, but place it front of the base station and use low-loss cables to place the antennas in various locations for measurements.
%We simply include it in the one-shot measurement of the base station channels (with transmit and receive gains adjusted according to antenna location) to estimate each of its antenna's channels to the BS.
